# Supplementary material for: Automating Thought of Search: A Journey Towards Soundness and Completeness
Source: arXiv:2408.11326 source file (2025-05-28)
Supplement: Supplementary file 2 [file appendix-b.tex]

\section{Model Correspondences}
We show one full correspondence with the language model per domain, LLM, and with or without partial successor soundness test.  The correspondences include {\em AutoToS prompt}, {\em Model response}, as well as {\em System messages} that log the current state of the system.

\subsection{24 Game}

\subsubsection{Deepseek-CoderV2}
\lstinputlisting[numbers=none,caption={Without partial successor soundness test}, label={lst:deepseek-coderv2-noval_logs}]{appendix/clean_logs/24game/deepseek-coderv2-noval_logs/clean_log.txt}
\lstinputlisting[numbers=none,caption={With partial successor soundness test}, label={lst:deepseek-coderv2-val_logs}]{appendix/clean_logs/24game/deepseek-coderv2-val_logs/clean_log.txt}

\subsubsection{GPT4-Mini}
\lstinputlisting[numbers=none,caption={Without partial successor soundness test}, label={lst:gpt4-mini-noval_logs}]{appendix/clean_logs/24game/gpt4-mini-noval_logs/clean_log.txt}
\lstinputlisting[numbers=none,caption={With partial successor soundness test}, label={lst:gpt4-mini-val_logs}]{appendix/clean_logs/24game/gpt4-mini-val_logs/clean_log.txt}

\subsubsection{GPT4}
\lstinputlisting[numbers=none,caption={Without partial successor soundness test}, label={lst:gpt4-noval_logs}]{appendix/clean_logs/24game/gpt4-noval_logs/clean_log.txt}
\lstinputlisting[numbers=none,caption={With partial successor soundness test}, label={lst:gpt4-val_logs}]{appendix/clean_logs/24game/gpt4-val_logs/clean_log.txt}

\subsubsection{Llama3.1 70B}
\lstinputlisting[numbers=none,caption={Without partial successor soundness test}, label={lst:llama3.1-70b-noval_logs}]{appendix/clean_logs/24game/llama3.1-70b-noval_logs/clean_log.txt}
\lstinputlisting[numbers=none,caption={With partial successor soundness test}, label={lst:llama3.1-70b-val_logs}]{appendix/clean_logs/24game/llama3.1-70b-val_logs/clean_log.txt}

\subsubsection{Llama3.1 405B}
\lstinputlisting[numbers=none,caption={Without partial successor soundness test}, label={lst:llama3.1-405b-noval_logs}]{appendix/clean_logs/24game/llama3.1-405b-noval_logs/clean_log.txt}
\lstinputlisting[numbers=none,caption={With partial successor soundness test}, label={lst:llama3.1-405b-val_logs}]{appendix/clean_logs/24game/llama3.1-405b-val_logs/clean_log.txt}

\subsection{BlocksWorld}

\subsubsection{Deepseek-CoderV2}
\lstinputlisting[numbers=none,caption={Without partial successor soundness test}, label={lst:deepseek-coderv2-noval_logs}]{appendix/clean_logs/blocks/deepseek-coderv2-noval_logs/clean_log.txt}
\lstinputlisting[numbers=none,caption={With partial successor soundness test}, label={lst:deepseek-coderv2-val_logs}]{appendix/clean_logs/blocks/deepseek-coderv2-val_logs/clean_log.txt}

\subsubsection{GPT4-Mini}
\lstinputlisting[numbers=none,caption={Without partial successor soundness test}, label={lst:gpt4-mini-noval_logs}]{appendix/clean_logs/blocks/gpt4-mini-noval_logs/clean_log.txt}
\lstinputlisting[numbers=none,caption={With partial successor soundness test}, label={lst:gpt4-mini-val_logs}]{appendix/clean_logs/blocks/gpt4-mini-val_logs/clean_log.txt}

\subsubsection{GPT4}
\lstinputlisting[numbers=none,caption={Without partial successor soundness test}, label={lst:gpt4-noval_logs}]{appendix/clean_logs/blocks/gpt4-noval_logs/clean_log.txt}
\lstinputlisting[numbers=none,caption={With partial successor soundness test}, label={lst:gpt4-val_logs}]{appendix/clean_logs/blocks/gpt4-val_logs/clean_log.txt}

\subsubsection{Llama3.1 70B}
\lstinputlisting[numbers=none,caption={Without partial successor soundness test}, label={lst:llama3.1-70b-noval_logs}]{appendix/clean_logs/blocks/llama3.1-70b-noval_logs/clean_log.txt}
\lstinputlisting[numbers=none,caption={With partial successor soundness test}, label={lst:llama3.1-70b-val_logs}]{appendix/clean_logs/blocks/llama3.1-70b-val_logs/clean_log.txt}

\subsubsection{Llama3.1 405B}
\lstinputlisting[numbers=none,caption={Without partial successor soundness test}, label={lst:llama3.1-405b-noval_logs}]{appendix/clean_logs/blocks/llama3.1-405b-noval_logs/clean_log.txt}
\lstinputlisting[numbers=none,caption={With partial successor soundness test}, label={lst:llama3.1-405b-val_logs}]{appendix/clean_logs/blocks/llama3.1-405b-val_logs/clean_log.txt}

\subsection{5x5 Crosswords}

\subsubsection{Deepseek-CoderV2}
\lstinputlisting[numbers=none,caption={Without partial successor soundness test}, label={lst:deepseek-coderv2-noval_logs}]{appendix/clean_logs/cw/deepseek-coderv2-noval_logs/clean_log.txt}
\lstinputlisting[numbers=none,caption={With partial successor soundness test}, label={lst:deepseek-coderv2-val_logs}]{appendix/clean_logs/cw/deepseek-coderv2-val_logs/clean_log.txt}

\subsubsection{GPT4-Mini}
\lstinputlisting[numbers=none,caption={Without partial successor soundness test}, label={lst:gpt4-mini-noval_logs}]{appendix/clean_logs/cw/gpt4-mini-noval_logs/clean_log.txt}
\lstinputlisting[numbers=none,caption={With partial successor soundness test}, label={lst:gpt4-mini-val_logs}]{appendix/clean_logs/cw/gpt4-mini-val_logs/clean_log.txt}

\subsubsection{GPT4}
\lstinputlisting[numbers=none,caption={Without partial successor soundness test}, label={lst:gpt4-noval_logs}]{appendix/clean_logs/cw/gpt4-noval_logs/clean_log.txt}
\lstinputlisting[numbers=none,caption={With partial successor soundness test}, label={lst:gpt4-val_logs}]{appendix/clean_logs/cw/gpt4-val_logs/clean_log.txt}

\subsubsection{Llama3.1 70B}
\lstinputlisting[numbers=none,caption={Without partial successor soundness test}, label={lst:llama3.1-70b-noval_logs}]{appendix/clean_logs/cw/llama3.1-70b-noval_logs/clean_log.txt}
\lstinputlisting[numbers=none,caption={With partial successor soundness test}, label={lst:llama3.1-70b-val_logs}]{appendix/clean_logs/cw/llama3.1-70b-val_logs/clean_log.txt}

\subsubsection{Llama3.1 405B}
\lstinputlisting[numbers=none,caption={Without partial successor soundness test}, label={lst:llama3.1-405b-noval_logs}]{appendix/clean_logs/cw/llama3.1-405b-noval_logs/clean_log.txt}
\lstinputlisting[numbers=none,caption={With partial successor soundness test}, label={lst:llama3.1-405b-val_logs}]{appendix/clean_logs/cw/llama3.1-405b-val_logs/clean_log.txt}

\subsection{ProntoQA}

\subsubsection{Deepseek-CoderV2}
\lstinputlisting[numbers=none,caption={Without partial successor soundness test}, label={lst:deepseek-coderv2-noval_logs}]{appendix/clean_logs/prontoqa/deepseek-coderv2-noval_logs/clean_log.txt}
\lstinputlisting[numbers=none,caption={With partial successor soundness test}, label={lst:deepseek-coderv2-val_logs}]{appendix/clean_logs/prontoqa/deepseek-coderv2-val_logs/clean_log.txt}

\subsubsection{GPT4-Mini}
\lstinputlisting[numbers=none,caption={Without partial successor soundness test}, label={lst:gpt4-mini-noval_logs}]{appendix/clean_logs/prontoqa/gpt4-mini-noval_logs/clean_log.txt}
\lstinputlisting[numbers=none,caption={With partial successor soundness test}, label={lst:gpt4-mini-val_logs}]{appendix/clean_logs/prontoqa/gpt4-mini-val_logs/clean_log.txt}

\subsubsection{GPT4}
\lstinputlisting[numbers=none,caption={Without partial successor soundness test}, label={lst:gpt4-noval_logs}]{appendix/clean_logs/prontoqa/gpt4-noval_logs/clean_log.txt}
\lstinputlisting[numbers=none,caption={With partial successor soundness test}, label={lst:gpt4-val_logs}]{appendix/clean_logs/prontoqa/gpt4-val_logs/clean_log.txt}

\subsubsection{Llama3.1 70B}
\lstinputlisting[numbers=none,caption={Without partial successor soundness test}, label={lst:llama3.1-70b-noval_logs}]{appendix/clean_logs/prontoqa/llama3.1-70b-noval_logs/clean_log.txt}
\lstinputlisting[numbers=none,caption={With partial successor soundness test}, label={lst:llama3.1-70b-val_logs}]{appendix/clean_logs/prontoqa/llama3.1-70b-val_logs/clean_log.txt}

\subsubsection{Llama3.1 405B}
\lstinputlisting[numbers=none,caption={Without partial successor soundness test}, label={lst:llama3.1-405b-noval_logs}]{appendix/clean_logs/prontoqa/llama3.1-405b-noval_logs/clean_log.txt}
\lstinputlisting[numbers=none,caption={With partial successor soundness test}, label={lst:llama3.1-405b-val_logs}]{appendix/clean_logs/prontoqa/llama3.1-405b-val_logs/clean_log.txt}

\subsection{Sokoban}

\subsubsection{Deepseek-CoderV2}
\lstinputlisting[numbers=none,caption={Without partial successor soundness test}, label={lst:deepseek-coderv2-noval_logs}]{appendix/clean_logs/sokoban/deepseek-coderv2-noval_logs/clean_log.txt}
\lstinputlisting[numbers=none,caption={With partial successor soundness test}, label={lst:deepseek-coderv2-val_logs}]{appendix/clean_logs/sokoban/deepseek-coderv2-val_logs/clean_log.txt}

\subsubsection{GPT4-Mini}
\lstinputlisting[numbers=none,caption={Without partial successor soundness test}, label={lst:gpt4-mini-noval_logs}]{appendix/clean_logs/sokoban/gpt4-mini-noval_logs/clean_log.txt}
\lstinputlisting[numbers=none,caption={With partial successor soundness test}, label={lst:gpt4-mini-val_logs}]{appendix/clean_logs/sokoban/gpt4-mini-val_logs/clean_log.txt}

\subsubsection{GPT4}
\lstinputlisting[numbers=none,caption={Without partial successor soundness test}, label={lst:gpt4-noval_logs}]{appendix/clean_logs/sokoban/gpt4-noval_logs/clean_log.txt}
\lstinputlisting[numbers=none,caption={With partial successor soundness test}, label={lst:gpt4-val_logs}]{appendix/clean_logs/sokoban/gpt4-val_logs/clean_log.txt}

\subsubsection{Llama3.1 70B}
\lstinputlisting[numbers=none,caption={Without partial successor soundness test}, label={lst:llama3.1-70b-noval_logs}]{appendix/clean_logs/sokoban/llama3.1-70b-noval_logs/clean_log.txt}
\lstinputlisting[numbers=none,caption={With partial successor soundness test}, label={lst:llama3.1-70b-val_logs}]{appendix/clean_logs/sokoban/llama3.1-70b-val_logs/clean_log.txt}

\subsubsection{Llama3.1 405B}
\lstinputlisting[numbers=none,caption={Without partial successor soundness test}, label={lst:llama3.1-405b-noval_logs}]{appendix/clean_logs/sokoban/llama3.1-405b-noval_logs/clean_log.txt}
\lstinputlisting[numbers=none,caption={With partial successor soundness test}, label={lst:llama3.1-405b-val_logs}]{appendix/clean_logs/sokoban/llama3.1-405b-val_logs/clean_log.txt}
